# Supplementary material for: DrivAerML: High-Fidelity Computational Fluid Dynamics Dataset for Road-Car External Aerodynamics
Source: arXiv:2408.11969 source file (2025-04-17)
Supplement: Supplementary file 1 [file appendix-mlevaluation.tex]

\clearpage
\section{ML evaluation}
\label{app:ml}
\subsection{Summary}

We have conducted preliminary analysis on our dataset using a modified version of one of the state-of-the-art scientific machine learning (SciML) methods, MeshGraphNet \cite{fortunato2022} on various tasks to illustrate the practicality of the dataset for ML evaluation.  We utilize the encoder-processor-decoder architecture in MeshGraphNets and modify the method to enable it to make time-averaged predictions \cite{ananthan2024}.  

The entire drivaer dataset is split into training (60\%), validation (20\%), and test (20\%) sets. For each use case, the model is trained on the training set, and the checkpoint that had the best validation error was used to obtain the inference results on the test set. 

For the DrivAer dataset, using the predicted surface pressure and wall-shear stress on the 8M node vtp surface mesh, we obtain predictions (shown in Figure \ref{fig:mlpredictions}) for the drag coefficient with a mean absolute percentage error (MAPE) of 0.032 and a mean absolute error (MAE): 0.009. For the lift coefficient the mean absolute error (MAE): 0.0164. The surface contours of the actual, predicted and error for the mean pressure and wall-shear stress are shown in Figure \ref{fig:mlpredictions3}. Training time is approximately 108 hours on x8 NVidia L40s GPUs and the inference time is less than a minute on the same hardware. Please note that these runs are preliminary and further work to optimize the methodology and hyperparameters is on-going which will published in future papers.

\vspace{0.025\textwidth}
\begin{figure}[htb]
     \centering
     \begin{subfigure}[b]{0.49\textwidth}
         \centering
         \includegraphics[width=\textwidth]{images/dataset/ml-cd-surface.png}
         \caption{Drag coefficient}
         \label{fig:mlcd}
     \end{subfigure}
     \hfill
     \begin{subfigure}[b]{0.49\textwidth}
         \centering
         \includegraphics[width=\textwidth]{images/dataset/ml-cl-surface.png}
         \caption{Lift coefficient }
         \label{fig:mlcl}
     \end{subfigure}
              \caption{Actual vs predicted for the force coefficients obtained through integration of the wall-shear stress and pressure}
    \label{fig:mlpredictions}
\end{figure}

\begin{figure}[htb]
     \centering
     \begin{subfigure}[b]{0.90\textwidth}
         \centering
         \includegraphics[width=\textwidth]{images/dataset/run0402_boundary_476_pMeanTrim.png}
         \caption{Mean pressure actual, prediction and error for a sample DrivAer run}
         \label{fig:mlpressure}
     \end{subfigure}
     \hfill
     \begin{subfigure}[b]{0.90\textwidth}
         \centering
         \includegraphics[width=\textwidth]{images/dataset/run0402_boundary_476_wallShearStressMeanTrim_dim0.png}
         \caption{Mean wall-shear stress actual, prediction and error for a sample DrivAer run}
         \label{fig:mlwss}
     \end{subfigure}
              \caption{Actual, Prediction and error for the mean pressure and wall-shear stress for a sample DrivAer unseen geometry}
    \label{fig:mlpredictions3}
\end{figure}

\newpage
